# Supplementary material for: Recursive Sketches for Modular Deep Learning
Source: arXiv:1905.12730 source file (2019-08-06)
Supplement: Supplementary file 1 [file repositoryappendix.tex]

\section{Benefits of sketch repository and the Modular view of the Network}
\subsection{Implicit Knowledge graph in the Sketch repository}

The collection of sketches form an implicit knowledge graph. When we think or ponder dream we may be doing a random walk on this implicit graph. This walk may be interleaved with computation using modules; that is, when a module fires, we may pull out related sketches in the neighborhood of the sketch that arises out of the module. The additional retrieved sketches may trigger the processing of another module. Thus the random walk/sketch graph exploration may be interleaved with triggering inputs into and firing of modules.

\subsection{Floating Modules}\label{sec:floatingm}

{\em Type/Class information can be identified from subspace components:}
Modules are more like program functions rather than blocks in a circuit that can't be shared across  different parts of the circuit. These functions listen in on specific subspaces (like ports) and if there is a match output something on another subspace (like a port).

each class/attribute is present in a subspace
looking for a subspace is like listening on a port for a class

if too many outputs at a layer then only top k are retained and others are compressed into a very small number of dimensions.

Can encode a very large network with O(d) size sketches and preserve information from cuts that are sparse, cuts smaller than O(d).

Gives protocol independent way of encoding class-structures into sketches.

<Diagram of comparison between communicating modules via neural edges and machines on a broadcast network> Maybe time multiplexing can be used to transfer larger amounts of information over the wires.

Examples of floating/shared modules:

A lines/curves sketcher can be used to sketch curves in images but also the curve representing speech.

A counting node can count number of copies of an object in an image or number of times a specific sound occurs. Thus a counting node has to be a "free floating" node

A clustering/dictionary learning module can be used in multiple places to find new concepts or to refine a concept. 

SQL-Projection-Groupby node. This may be used to take a set of sketches and project out a specific field such as color or texture or velocity and group the sketches by different values. A counting node may then be applied to compress a sketch with repetitions into a (count, repeated value) sketch. 

Such algebraic nodes can be used to simplify a sketch/input into an expression tree/dag. 

Modules listen in on a subspace. This can be thought of as a select operation with a where statement that is looking for specific features. Such modules can also be thought of as hardwired modules. 

Derived classes are ancestor modules of the parent class: The recursive sketch of the derived class will automatically be similar to sketch of the parent class.

\subsubsection{Identifying motion patterns as curves in sketch space}
We will show how a butterfly flapping its wings, or a person walking, or a snake slithering on the ground can be identified using this modular view and sketching. Consider a video of a butterfly flapping its wings at a fixed location. Each video frame produces a sketch identifying the butterfly and outputs attributes corresponding it its color, shape, position and orientation of wings. Across video frames all that changes is orientation and position of wings. So over time we get a curve in sketch space. Since the video is periodic the curve is actually a loop. Now if we have a module to sketch curves, such a module could take this curve and sketch it into its top few coefficients in say a polynomial/fourier representation. So the final coefficient sketch would correspond to a flying butterfly. Similar things can happen for any periodic motion such as a person walking (which is periodic once you subtract the velocity vector) or a snake slithering (a periodic motion). Each of these is a specific type of loop in sketch space. In fact this may even be done unsupervised: The sketch of a flying butterfly will form a new cluster center in sketch space and can be identified as a new module (see below).

\subsection{Sketch Repository is used in adding new classification modules}\label{sec:addingmodules}

Claim 5 shows that sketches are "far apart" unless they represent similar objects. So it is likely that all the objects that correspond to a given module are all near each other and form a cluster. Thus if we look at the sketch space, we may find a new cluster and we may learn this cluster as a new module.

Given an input, we store a sketch of all the outputs of the strong classifiers.

Having feature sketches helps in clustering features to form a new module. For example all related features may have the same color or the same texture or form a strongly connected component. 

A collection of possibly floating strong classifiers: A strong classifier is something that can reconstruct the input sketches to high degree of accuracy. It may append a sketch of the inputs that has a high similarity to the inputs. This makes it easier for indexing and retrieval so that the detailed sketch of inputs can be retrieved from the output of the strong classifier.

To form a new strong classifier: First find a cluster of sketches by either projection (such as moving objects on road project on "moving" , "on - road" to learn cars, trucks, motorcycles, or has "eyes" "nose" "mouth", "hands") or by finding sketches related to a given sketch. This allows semi supervised learning. This can give a weak classifier for an object. Then objects that match this weak classifier can be learnt strongly recursively to learn detailed features (like hairstyles, dress styles, ) This can be used to then identify a person holding an object, subtract the person and classify the object.

The sum part of the sketch can directly be used to find the total amt of each color. By extraxcting the color subspace one can cluster and then groupby color

There maybe sketches resistant to permutations

Infact just averaging a set of sketches tells u the dominant direction. Doing k means will give a few directions. It is what u would have got from original data. The sketching preserves it. Maybe keep a matrix sketch to preserve distribution using sampling or random projection rather than keeping all sketches

If the seq vector of sketches is changing smoothly this automatically goes to a curve analyzer.thus curve analyzer is a floating module. An object or bug transforming smoothly can go to a curve analyzer. A butterfly flapping its wings will produce a periodic curve in sketch space. Similarly a ball bouncing or man walking. So such curve analyzer, periodicity detector needs to be shared. Discontinuity in curve will emit a token/word. Similarly discontinuity in highever level seq of sketches will produce language based description of the scene

Another example of separability may just be pure factoring for example many parts moving together factors naturally into [sketch of parts] x [sketch of motion]
or [sketch of parts] x [sketch of color/texture]

samy paper on high margin clssifier
pushmeet /niru paper on semantic segmentation via rnn

Sql project sum becomes a subspace operator.

The sketch itself can be used to suggest the next simplifying operator.
 
If there are sufficiently many sparse firings involving each node. Then network can be learned
